# Supplementary material for: ELiTe: Efficient Image-to-LiDAR Knowledge Transfer for Semantic Segmentation
Source: arXiv:2405.04121 source file (2024-05-07)
Supplement: Supplementary file 1 [file supp_vis.pdf]

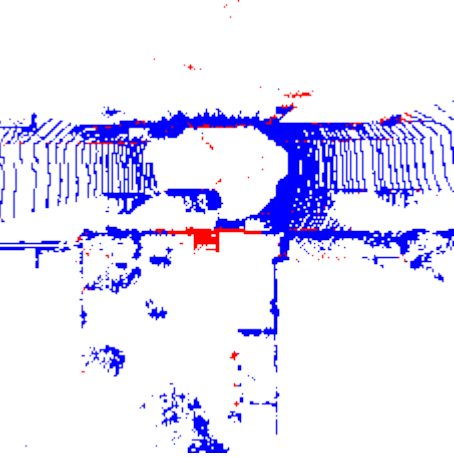

**(a) Baseline Error**

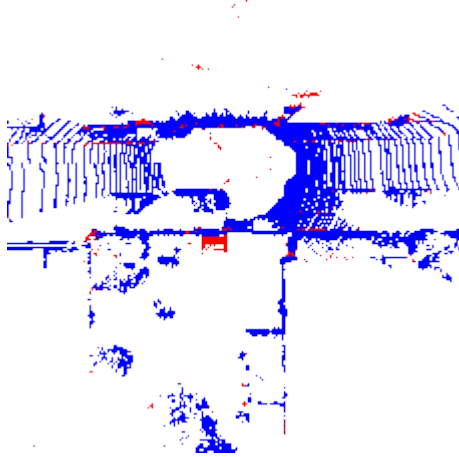

**(b) ELiTe Error**

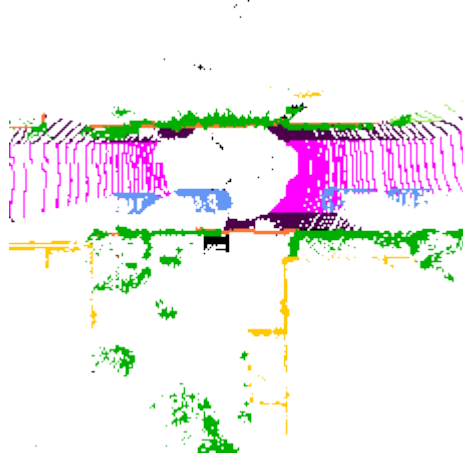

**(c) Ground Truth**
